# Supplementary material for: Unraveling the nature of magnetism of the 5$\boldsymbol{d^4}$ double perovskite Ba$_2$YIrO$_6$
Source: arXiv:1805.05243 source file (2018-06-11)
Supplement: Supplementary file 1 [file Supplement_revision.pdf]

# Unraveling the nature of magnetism of the $5d^4$ double perovskite $Ba_2YIrO_6$
*Supplemental Information*

S. Fuchs,[1,2] T. Dey,[1] G. Aslan-Cansever,[1,2] A. Maljuk,[1] S. Wurmehl,[1] B. Büchner,[1,2] and V. Kataev[1]
[1]*Leibniz Institute for Solid State and Materials Research IFW Dresden, D-01171 Dresden, Germany*
[2]*Institut für Festkörper- und Materialphysik, Technische Universität Dresden, D-01062 Dresden, Germany*

## STATISTICAL ANALYSIS OF THE DISTRIBUTION OF MAGNETIC CENTERS

### Numerical simulations

For a better understanding of the experimental results we have performed numerical simulations of the statistical distribution of paramagnetic centers in $Ba_2YIrO_6$ as a function of their concentration $n$ and analyzed the dependence of the average distance between the defects on $n$ and the formation of clusters and the evolution of their size as a function of $n$. A cluster is defined as a group of magnetic defects interacting over a given distance, and the cluster size means the number of such defects in the group.

The double perovskite (DP) structure $A_2BB'O_6$ can be understood as the superposition of two interpenetrating simple perovskite (SP) lattices $ABO_3$ and $AB'O_3$, i.e., if $B = B'$ it reduces to the pervoskite lattice $ABO_3$. The majority of paramagnetic species giving rise to magnetism of $Ba_2YIrO_6$ were identified in the ESR experiments with $Ir^{4+}$ ($S = 1/2$) and $Ir^{6+}$ ($S = 3/2$) centers. If these centers reside exclusively on the $B' = Ir$ sites of the DP lattice then the shortest exchange interaction path $p_1$ would involve two oxygen bridges Ir–O–O–Ir, and the next one $p_2$ could involve the $Y^{3+}$ nonmagnetic site, Ir–O–Y–O–Ir [1]. If, however, these centers may occupy both B′ and B sites then the shortest exchange path $p_0$ would be between the two neighboring corner-sharing octahedra $B'O_6$ and $BO_6$. In this case, the problem reduces to the on the SP lattice. For completeness, one can also define a direct geometrical distance $d$ between two spin centers which could be relevant for dipole-dipole interaction.

The algorithm of the simulation program includes the random filling up with a given percentage of defects $n$ an $N^3$ cubic lattice with the edge length of $N = 51$ sites. The lattice could be either DP or SP where the average smallest distance $D_{\rm av}$ between the defects in the relevant units $p_{\rm i}$ ($i = 0, 1, 2$) or $d$ is calculated in the next step. To improve the statistics, the simulation is repeated several times and the results are averaged.

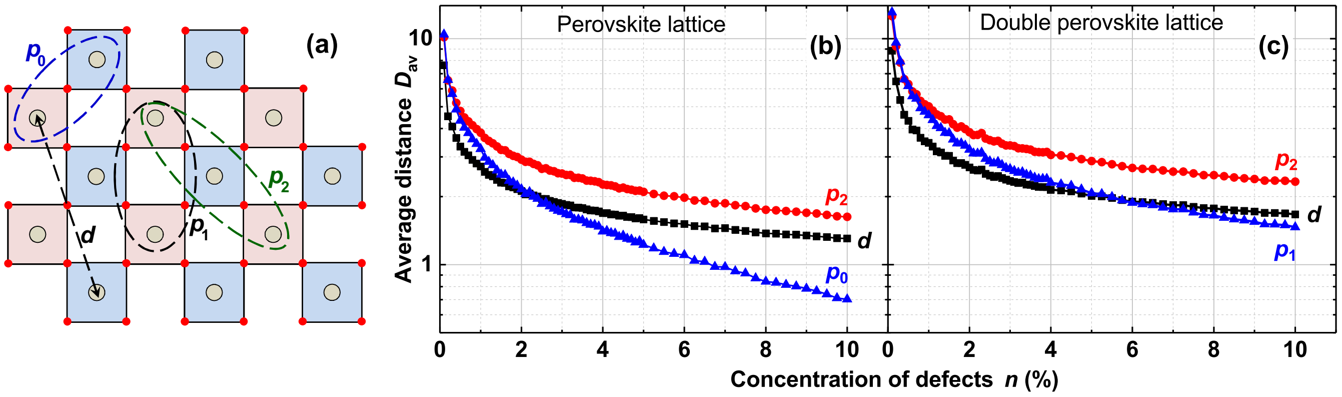


FIG. S1: (a) Definition of exchange path units in the DP lattice $A_2BB'O_6$: between nearest corner shared octahedra $B'O_6$ and $BO_6$ – $p_0$; via two oxygen bridges B′–O–O–B′ – $p_1$ ; via the bridge B′–O–B–O–B′ – $p_2$; $d$ is the geometrical distance between two selected sites; Average distance between the defects in an SP (b) and DP (c) lattice as a function of the defect concentration $n$ for four differently defined distance units $p_0$, $p_1$, $p_2$ and $d$. Solid lines are guide for the eye. (see the text)

In Fig. S1 the average distance $D_{\rm av}$ between the defects in the above introduced definitions of the distance units is plotted as a function of the defect concentration $n$ for SP and DP lattices. As expected, $D_{\rm av}$ shrinks with increasing $n$. Interestingly, it drops down very fast in the range $0 < n \lesssim 2\,\%$ and then decreases smoothly further for higher $n$. In the SP lattice with $2\,\%$ of defects, $D_{\rm av}$ amounts to two shortest exchange path units $p_0$, whereas in the DP lattice with the shortest exchange path $p_1$, one reaches $D_{\rm av} = 2p_1$ at $n = 5.5\,\%$ only. To illustrate the distribution of the defect centers, we show in Fig. S2 examples of the stochastic filling of an SP lattice with defects for three values of $n$.

Defect centers which generally can occur at every site are visualized as small colored spheres. Spheres with the same color are connected via exchange path of the same length. The number of particles with shorter interaction lengths rapidly grows with $n$, as expected.

Fig. S3 visualizes the formation of clusters on the SP lattice with increasing the concentration of defects $n$. Defects are depicted as small differently colored spheres. Defects belonging to the same cluster have the same color. The color itself has no special meaning and is chosen randomly for different clusters. While at the smallest concentration of $2\,\%$ there are practically no clusters formed, they become appreciable at $n = 4\,\%$, and at $n = 10\,\%$ almost all defects are coupled in one cluster.

Fig. S4 presents the results of the cluster analysis where several relevant quantities obtained from the simulations are plotted as a function of the concentration of the paramagnetic centers $n$. The distance between the neighboring centers in a cluster is defined in exchange path units $p_0$, $p_1$ and $p_2$, respectively. In panel (a) the number of clusters in the lattice is normalized to the number of total lattice sites available for the defects $N_{\mathrm{cl}}^{\mathrm{norm}}$. At small $n$, the number of defects increases without forming any clusters. At a certain concentration, the clusters begin to form and their number grows with further increasing $n$. However, above some specific concentration of defects, which depends on

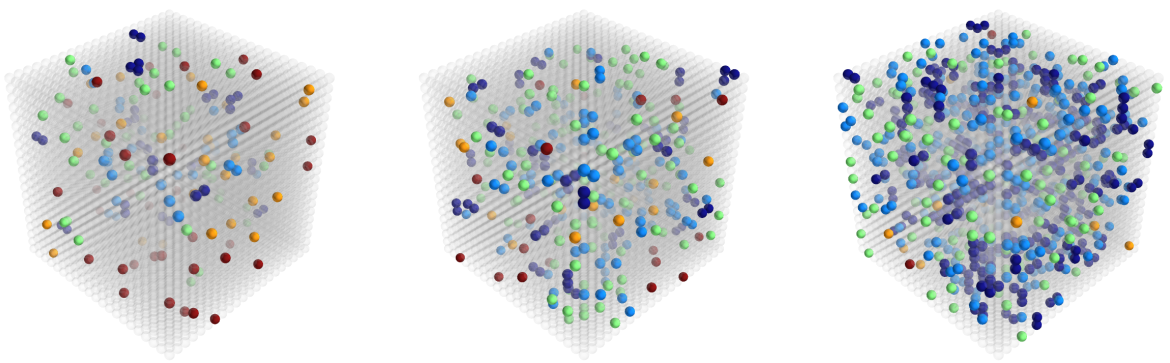

(a) 2 % (b) 4 % (c) 10 %

FIG. S2: Examples of the distribution of defects (colored spheres) on an SP lattice with the edge length of $N = 21$ sites for three selected concentrations $n$. The color identifies the defects having the same distance to the nearest neighbor defined in the units of the exchange path $p_0$: dark blue$\,=p_0$; light blue$\,=2p_0$; green$\,=3p_0$; orange$\,=4p_0$, and red$\,\geq 5p_0$. (see the text)

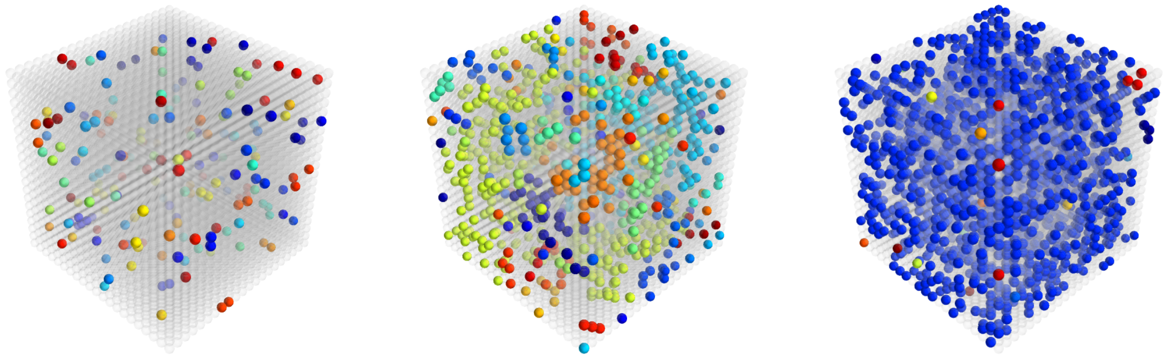

(a) 2 % (b) 4 % (c) 10 %

FIG. S3: Examples of the clustering of defects (colored spheres) on an SP lattice with the edge length of $N = 21$ sites with increasing their concentration $n$. The defects are connected in a cluster by the maximum exchange path length of $2p_0$. Defects belonging to the same cluster have the same color. (a) $n = 2\,\%$, practically all defects are independent; (b) $n = 4\,\%$, defects are coupled in mid-size clusters; (c) $n = 10\,\%$, practically all defects belong to the same cluster.

the chosen interaction distance between the defects in the cluster ($p_0$, $2p_0$, $p_1$, or $2p_1$) and the type of the lattice (SP or DP), the number of clusters decreases since more and more defects are joining the same cluster. Panel (b) depicts the concentration dependence of the average cluster size $S_{\rm av}$. Remarkably, $S_{\rm av}$ grows exponentially with $n$ for all types of interaction distances. Panel (c) shows the dependence on $n$ of the size of the largest cluster normalized to the number of all defects $S_{\rm max}^{\rm norm}$. The value of 1 means that all defects belong to one cluster. It is instructive to define a threshold concentration $n_{\rm th}$ at which $S_{\rm max}^{\rm norm} = 0.5$ meaning that one half of the defects belongs to the largest cluster. The average cluster size at the concentration $n_{\rm th}$ amounts to $\approx 8(\pm 1)$ irrespective of the chosen interaction distance [Fig. S4(b)].

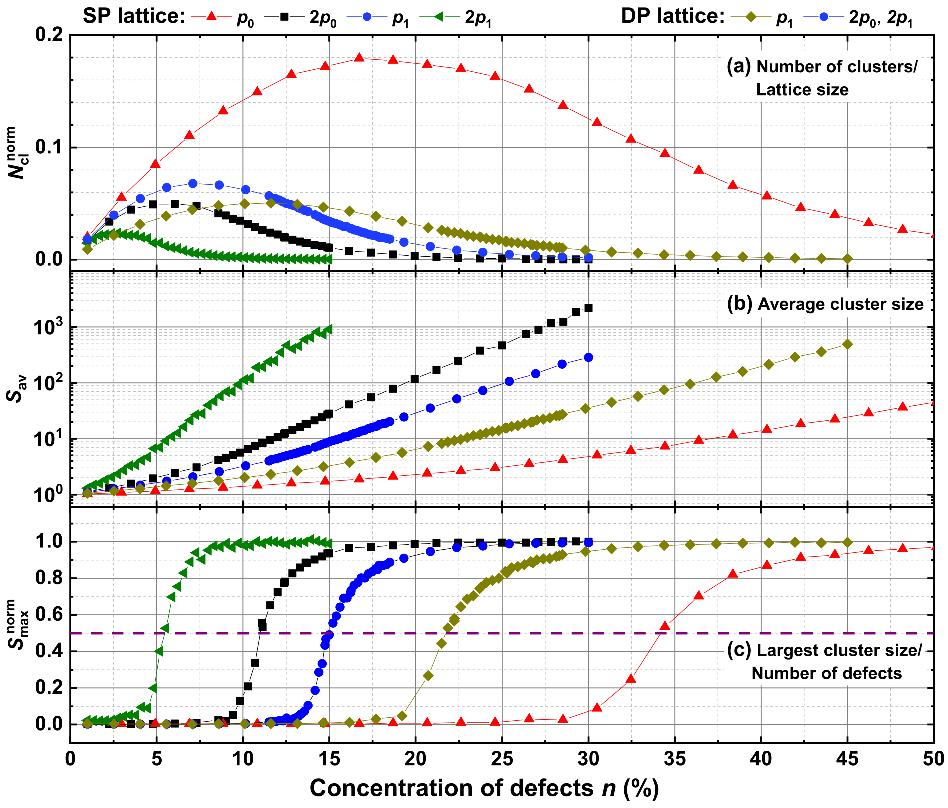


FIG. S4: Results of the cluster analysis for SP and DP lattice for three differently defined distance units $p_0$, $p_1$ and $p_2$. Dependence on the defect concentration $n$ of: (a) number of clusters normalized to the number of total lattice sites $N_{\rm cl}^{\rm norm}$; (b) average cluster size $S_{\rm av}$; (c) size of the largest cluster normalized to the number of all defects $S_{\rm max}^{\rm norm}$. Horizontal dashed line in (c) indicates the level at which one half of all defects in the lattice belongs to the largest cluster. The corresponding threshold concentration $n_{\rm th}$ where the line intersects the curves depends on the distance between the centers in the cluster. Solid lines are guides for the eye. (see the text)

## Discussion

According to the above analysis, the full percolation in the DP lattice is achieved at the concentration of defects in the range 20 - 30 % depending on the length of the chosen exchange path $p_1$ or $2p_1$ [Fig. S4(c)]. For the case of the SP lattice it reduces to 8 - 20 %, respectively. Since the samples studied in the present work do not order magnetically and the concentration of magnetic centers is relatively small ($\sim 4\,\%$), the situation is far away from the full percolation. Still, magnetic correlations are evident from susceptibility and ESR data. This supports theoretical ideas of long-range character of superexchange in the 5$d$ DP compounds [1, 2] whereas some antisite Y $\leftrightarrow$ Ir disorder might also play a role [3]. Significant antisite disorder which effectively reduces the interactions between magnetic centers to the case of the SP lattice with shorter exchange paths might help to rationalize the occurrence of magnetic order in "stronger magnetic" samples. However, at least in the case of "weaker magnetic" samples studied in the present work it remains an open question if one could treat $Ba_2YIrO_6$ as a simple perovskite.

[1] S. Kanungo, B. Yan, C. Felser, and M. Jansen, Phys. Rev. B **93**, 161116 (2016).
[2] X. Ou, Z. Li, F. Fan, H. Wang, and H. Wu, Sci. Rep. **4** (2014), 10.1038/srep07542.
[3] Q. Chen, C. Svoboda, Q. Zheng, B. C. Sales, D. G. Mandrus, H. D. Zhou, J.-S. Zhou, D. McComb, M. Randeria, N. Trivedi, and J.-Q. Yan, Phys. Rev. B **96**, 144423 (2017).
